# Supplementary material for: Universal Streaming of Subset Norms
Source: arXiv:1812.00241 source file (2020-04-05)
Supplement: Supplementary file 1 [file appendix.tex]

\section{Missing Proofs from Section~\ref{sec:HHexamples}}
\label{app:HHexamples}

%%% Local Variables: 
%%% mode: latex
%%% TeX-master: "writeup"
%%% End: 
